# Supplementary material for: Event-based Continuous Color Video Decompression from Single Frames
Source: arXiv:2312.00113 source file (2026-10-05)

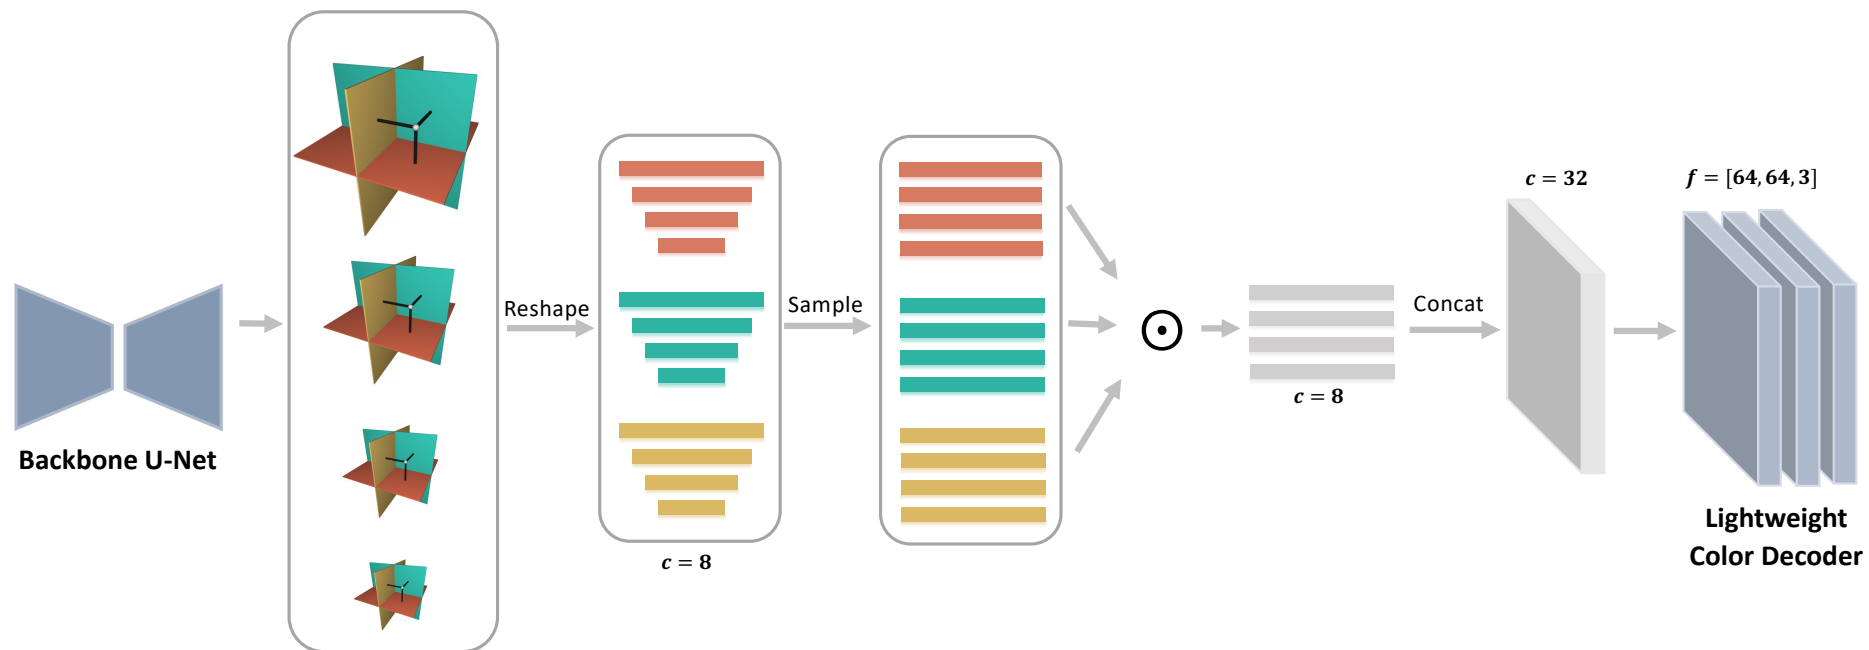

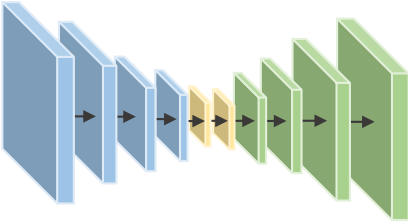

Supplement: Supplementary file 1 [file supp_pipeline.pdf]
